# Supplementary material for: Generating Band-Limited Adversarial Surfaces Using Neural Networks
Source: arXiv:2111.07424 source file (2021-11-14)
Supplement: Supplementary file 1 [file appendices.tex]

% Writing appendices is super super easy in LaTeX. You just write
% \appendix to demarcate where the normal content ends and the appendices start. After \appendix, chapters (started with \chapter) are considered as appendices.
%
% In this example though, we're using the appendices environment. Long story short, this is because we want some fancy titles in the toc.
\begin{appendices}

% Appendix A
% ----------

\chapter{Some random python code}
This template includes the \texttt{minted} package, which allows you to import code and syntax highlight it. For example, the text below is imported directly from the \texttt{code/test.py} file using the \textbackslash\texttt{inputminted} command:

\begin{framed}
\inputminted{python}{code/test.py}
\end{framed}

And here is a snippet of Python with the \texttt{minted} environment:

\begin{framed}
\begin{minted}[breaklines]{python}
# Why don't you try running this?
# See what it does? hm?

m = [ 2, 3, 0, 1, 4 ];
x = [ 'rmdq', 'd', 'n`slk', 'odftp`v)', 'hdk' ];

c = ''.join(list(map(lambda y: chr(ord(y) ^ 5).upper() + ' ' if y != ' ' else '  ', ' '.join([ x[m[i]] for i, v in enumerate(x) ]))));

print('%s\r\n%s\r\n%s\r\n' % ('=' * len(c), c, '=' * len(c)));
\end{minted}
\end{framed}

\cleardoublepage
Minted supports many, many languages -- so you're not just limited to Python. For example, here's some random C++ code.

\begin{framed}
\begin{minted}[breaklines]{cpp}
void CTimesTable::Print(const int number, const int upTo) const
{
    for(int i = 1; i <= upTo; i++)
        printf("%d x %d = %d\r\n", number, i, number * i);
}
\end{minted}
\end{framed}

% Appendix B
% ----------

\chapter{Some other stuff}
Here is just an example of some other stuff.

% End of appendices
\end{appendices}
